# Supplementary material for: Shared Adversarial Unlearning: Backdoor Mitigation by Unlearning Shared Adversarial Examples
Source: arXiv:2307.10562 source file (2023-07-20)
Supplement: Supplementary file 1 [file extension.tex]

\subsection{Extension to Multiple Targets}

\paragraph{Extension to Universal adversarial perturbation.} As shown in the \cite{chai2022oneshot, zeng2022adversarial}, Universal Adversarial Perturbation (UAP) achieve excellent performance in backdoor defense. We remark that the proposed theorem and method also fit adversarial training with UAP. By replacing the individual perturbation for each sample with a UAP, we can reach a UAP version of our method and the shared universal perturbation risk is smaller than the vanilla  universal risk. More details for this case are left in the Appendix.

\paragraph{Target case} Up to now, we assume that $\hat{y}$ is not accessible. Since there is already much work on target label detection on the backdoor attack, we now extend our method to cases where the target label $\hat{y}$ is known.

Given $\hat{y}$, the targeted shared adversarial risk can be defined as 
\begin{equation}
    \label{eq::cup_target}
    \begin{aligned}
    \hat{\gR}_{sa}(\htt) &= \frac{\sum_{i=1}^N \max_{\veps_i \in \gS}\ind\left(\htt(\tilde{\vx}_i(\veps_i))=\hat{y}, \htt(\tilde{\vx}_i(\veps_i)) = \hbd(\tilde{\vx}_i(\veps_i)), y_i\neq \hat{y}\right)}{\sum_{i=1}^N \ind(y_i\neq \hat{y})}
    \end{aligned}
\end{equation}
\begin{theorem}
Under Assumption~\ref{assm:S}, for a classifier $\htt$, we have
$$\gR_{bd}(\htt) \leq \hat{\gR}_{sa}(\htt) \leq \gR_{mix}(\htt).$$

\end{theorem}

After similar relaxation in Section \ref{sec::loss}, we can reach the targeted objective by replacing the untargeted adversarial training with targeted adversarial training.  More details for this case are left in the Appendix.

\paragraph{Extension to Targeted Adversarial training} A simple way to find shared adversarial examples for $\hbd$ and $\htt$ in the Maximization step is utilizing targeted adversarial attack  with random target labels. To do so, we consider the following loss function in the maximization step:
\begin{equation}
    \ell_5(\vtheta,(\tilde{\vx}_i(\veps_i),y_i)) = -\text{CE}(\vp(\tilde{\vx}_i(\veps_i),\vtheta),\bar{y}_i)- \text{CE}(\vp(\tilde{\vx}_i(\veps_i),\vtheta_{bd}),\bar{y}_i).
\end{equation}
where $\bar{y}_i$ is a randomly selected pseudo target label and $\bar{y}_i\neq y_i$.
